# Supplementary material for: Data-Dependent Coresets for Compressing Neural Networks with Applications to Generalization Bounds
Source: arXiv:1804.05345 source file (2019-05-18)
Supplement: Supplementary file 1 [file ADAPTIVE-appendix_empirical.tex]

\subsection{Analytical Results for Section~\ref{sec:analysis_empirical} (Empirical Sensitivity)}
\label{app:analysis_empirical}
% We begin by stating the formal definition of the relative importance of an incoming edge $\edge \in [\eta^{\ell-1}]$ to a neuron $\neuron \in [\eta^\ell]$ in layer $\ell \in \compressiblelayers$.
% \begin{definition}[Relative Importance]
% For a point $\Point \in \supp$ and a neuron $\neuron \in [\eta^\ell]$ in the $\ell^\text{th}$ layer, define the importance functions $\g{\Input}$ for each incoming positive edge as
% $$
% \g{\Input} = \g{\Input} \qquad \forall{\edge \in \Wpm},
% $$
% and similarly define the importance function $\gMin{\Input}$ over negative edges $\edge \in \Wminus$.
% % and 
% % $$
% % \gMin{\Input} = \gMinus{\Input} \qquad \forall{\edge \in \Wminus}.
% % $$
% \end{definition}
Recall that the sensitivity $\s[\edge]$, of an edge $\edge \in \Wpm$ is defined as the maximum (approximate) relative importance over a subset $\SS \subseteq \PP \iid \DD^n$, $\abs{\SS} = n'$ (Definition~\ref{def:empirical-sensitivity}). We now establish a technical result that quantifies the accuracy of our approximations of edge importance.

\subsection{Order Statistic Sampling}
% Let $X \sim \DD$ be a random variable with $\supp = [0, 1]$, Cumulative Distribution Function (CDF) and probability density function, denoted by $F(\cdot)$ and $p(\cdot)$, respectively. Let $M = \min \{x \in [0,1] : F(x) = 1\}$ and recall that $\eta$ and $\eta^*$ denote the total number of neurons in the neural network and the maximum number of neurons per layer, respectively.

% Let $\SS = \{X_1, \ldots, X_n\} \iid \DD^n$ be a set containing $n$ random variables and let $\FF$ be the (failure) event that $C \max_{X \in \SS} X < X_{n+1}$ for $C \ge 9 \, K \in [18, 9 \, \kmax]$. We now proceed to state our core technical result that bounds the probability of event $\FF$ for distributions satisfying the CDF condition presented in Assumption~\ref{asm:cdf}, and for any desired failure probability $\delta \in (0,1)$, provides a lower bound on the number of samples $n = |\SS|$ required to ensure that $\Pr(\FF) \leq \delta$.
% \LL{I feel like the above paragraph is redundant since it is restated more concisely in the lemma below.}

\begin{lemma}
\label{lem:order-statistic-sampling}
Let $C \ge 2$ be a constant and $\DD$ be a distribution with CDF $F(\cdot)$ satisfying $F(\nicefrac{M}{C}) \leq \exp(-1/K)$ where $K \in \Reals_+$ is a universal constant and $M = \min \{x \in [0,1] : F(x) = 1\}$. Let $\SS = \{X_1, \ldots, X_n\}$ be a set of $n = |\SS|$ independent and identically distributed (i.i.d.) samples each drawn from the distribution $\DD$. Let $X_{n+1} \sim \DD$ be an i.i.d. sample. Then,
\begin{align*}
    \Pr \left(C \, \max_{X \in \SS} X \leq X_{n+1} \right) \leq \exp(-n/K) 
    %\leq \exp \left(-\frac{n}{\kmax}\right)
\end{align*}
%where $K \leq \kmax$ is a constant as in Assumption~\ref{asm:cdf}.
% Moreover, for any $\delta \in (0, 1)$ if the size of $\SS$ satisfies
% $$
% n = |\SS| \ge \ceil*{\log(1 / \delta) \kmax},
% $$
% then the probability of event $\FF$ is bounded above by $\delta$, i.e., $\Pr(\FF) \leq \delta$.
\end{lemma}
\begin{proof}
Let $\xmax = \max_{X \in \SS}$ and let $\FF$ denote the failure event $C \, \xmax < X_{n+1}$. Then,
\begin{align*}
\Pr(\FF) &= \Pr(C \, \xmax < X_{n+1}) \\
&= \int_{0}^M \Pr(\xmax < \nicefrac{x}{C} | X_{n+1} = x) \, p(x) \, dx \\
&= \int_{0}^M \Pr\left(X < \nicefrac{x}{C} \right)^n \, p(x) \, dx &\text{since $X_1, \ldots, X_n$ are i.i.d.} \\
%
% &\leq \Pr(X \leq \nicefrac{M}{C})^n \int_0^M p(x) \, dx \\
%
&\leq \int_{0}^M F(\nicefrac{x}{C})^n \, p(x) \, dx &\text{where $F(\cdot)$ is the CDF of $X \sim \DD$} \\
&\leq  F(\nicefrac{M}{C})^n \int_{0}^M p(x) \, dx &\text{by monotonicity of $F$} \\
&= F(\nicefrac{M}{C})^n \\
&\leq \exp(-n/K)  &\text{CDF Assumption},
\end{align*}
and this completes the proof.
 \LL{I am worried that the pdf does not always exist. Igor and I discussed that (and we could double-check with him) but if we skip the integrals involving the pdf, we can just formulate it as Lebesgue integral, such that we don't need to ever rely on the pdf.} \CB{How about the new version of the proof (above) which doesn't use Riemann-Stieltjes? I'm not sure whether this fixes the problem, but at least there is no Riemann-Stieltjes.}

\end{proof}

\subsection{Case of Positive Weights}
In this subsection, we establish approximation guarantees under the assumption that the weights are strictly positive. The next subsection will then relax this assumption to conclude that a neuron's value can be approximated well even when the weights are not all positive.

% \LL{Here, we call the (n+1)th sample x', above it's $X_{n+1}$. Maybe one version everywhere}
% \LL{Also the 9 here is confusing, because it is not used anywhere as of now} \CB{But it is used? (see proof of Theorem~\ref{thm:sensitivity-approximation}}
% Let $C = 9 \kmax \ge 9 K$ be a constant. For $\Point \sim \DD$, let $\Aplus$ denote the event 
% $$
% \forall{\edge \in \Wpm}, \qquad  C \, \sPl = C \, \max_{\Point' \in \SS} \g{\Input'} \ge \g{\Input},
% $$
% and similarly let $\Aminus$ denote the event 
% $$
% \forall{\edge \in \Wmi}, \qquad C \, \sMi = C \, \max_{\Point' \in \SS} \gMin{\Input'} \ge  \gMin{\Input}.
% $$
Let $C = 9 \kmax \ge 9 K$ be a constant. We would like to apply Lemma~\ref{lem:order-statistic-sampling} in conjunction with Assumption~\ref{asm:cdf} to conclude that a logarithmic (in $1/\delta$ and $\eta \cdot \eta^*$) sized $\SS \subseteq \PP$ suffices to obtain $\Pr_{\Input \sim \DD}(C \, \s < \gHat{\Input}) \leq \delta$. However, Assumption~\ref{asm:cdf} is defined with respect to the CDF of $\g{\Input}$, denoted by $\cdf{\cdot}$, and \emph{not} that of $\gHat{\Input}$, denoted by $\cdfHat{\cdot}$. To bridge this gap, we establish the following technical result that relates the CDF of $\gHat{\Input}$ to that of $\g{\Input}$, provided that $\hat a^{\ell -1}(\Input) \in (1 \pm \epsilon) a^{\ell}(\Input)$. 
% For $\Point \sim \DD$, any layer $\ell \in \compressiblelayers$, and neuron $\neuron \in [\eta^\ell]$, let $\cdf{\cdot}$ and $\cdfHat{\cdot}$ denote the CDF of the random variables $\g{\Input}$ and $\gHat{\Input}$, respectively.
\begin{lemma}
\label{lem:cdf-relationship}
Let $\epsilon \in (0,1/2)$, $\ell \in \compressiblelayers$. Let $\Point \sim \DD$ be a randomly drawn point and assume that $\hat a^{\ell-1}(\Point) \in (1 \pm \epsilon) a^{\ell-1}(\Point)$. Then, for all $\edge \in \Wpm \subseteq [\eta^{\ell-1}]$ and for any constant $\gamma \in [0,1]$,
\begin{align*}
\cdf{\gamma/3} \leq \cdfHat{\gamma} \leq \cdf{3\gamma}.
\end{align*}
\end{lemma}
\begin{proof}
Let $\Point \sim \DD$ be a randomly drawn point and let $\edge \in \Wpm$ be arbitrary. By definitions of the CDF and $\g{\Input}$, we have
\begin{align*}
\cdfHat{\gamma} &= \Pr \left( \gHat{\Input} \leq \gamma \right) \\
&= \Pr \Big( \gHatDef{\Input} \leq \gamma \Big) \\
&= \Pr \Big( \WWRowCon_\edge \, \hat a_{\edge} (\Point) \leq \gamma \, \sum_{\idx \in \Wpm} \WWRowCon_\idx \, \hat a_{\idx}(\Point) \Big) \\
&= \Pr \Big( \WWRowCon_\edge \, \hat a_{\edge}(\Point) \leq \gamma \, \sum_{\idx \in \Wpm \, : \, \idx \neq \edge} \WWRowCon_\idx \, \hat a_{\idx}(\Point) + \gamma \WWRowCon_\edge \, \hat a_{\edge}(\Point) \Big).
\end{align*}
Define $\hat{\Sigma}_{(-j)} = \sum_{\idx \in \Wpm \, : \, \idx \neq \edge} \WWRowCon_\idx \, \hat a_{\idx}(\Point)$ and $\Sigma_{(-j)} = \sum_{\idx \in \Wpm \, : \, \idx \neq \edge} \WWRowCon_\idx \, a_{\idx}(\Point)$ for notational brevity. Note that since $\hat a^{\ell-1}(\Point) \in (1 \pm \epsilon) a^{\ell-1}(\Point)$, we have
\begin{align*}
\hat{\Sigma}_{(-j)} &= \sum_{\idx \in \Wpm \, : \, \idx \neq \edge} \WWRowCon_\idx \, \hat a_{\idx}(\Point) \\
&\leq (1 +\epsilon)  \sum_{\idx \in \Wpm \, : \, \idx \neq \edge} \WWRowCon_\idx \, a_{\idx}(\Point) \\
&= (1 + \epsilon) \Sigma_{(-j)}.
\end{align*}
Equipped with this inequality, we continue from above by rearranging the expression
\begin{align*}
\cdfHat{\gamma} &= \Pr \Big( (1 - \gamma) \WWRowCon_\edge \, \hat a_{\edge}(\Point)  \leq \gamma \, \hat{\Sigma}_{(-j)} \Big) \\
&\leq \Pr \Big( (1 - \gamma) \WWRowCon_\edge \, \hat a_{\edge}(\Point)  \leq \gamma \, (1 + \epsilon) \Sigma_{(-j)} \Big) \\
&\leq  \Pr \Big( (1 - \gamma) (1- \epsilon) \WWRowCon_\edge \,  a_{\edge}(\Point)  \leq \gamma \, (1 + \epsilon) \Sigma_{(-j)} \Big),
\end{align*}
where in the last inequality we used the fact that $a_{\edge} (1-\epsilon) \leq \hat a_{\edge}$ by assumption of the lemma. Moreover, since $\epsilon \in (0,1/2)$, observe that the ratio $\nicefrac{1 + \epsilon}{1 - \epsilon} \leq 3$. Dividing both sides by $1 - \epsilon$ in the expression above and applying this inequality we obtain
\begin{align*}
%\Pr \Big( (1 - \gamma) (1- \epsilon) \WWRowCon_\edge \,  a_{\edge}(\Point)  \leq \gamma \, (1 + \epsilon) \Sigma_{(-j)} \Big)
\cdfHat{\gamma} &\leq \Pr \Big( (1 - \gamma)  \WWRowCon_\edge \,  a_{\edge}(\Point)  \leq 3 \gamma  \, \Sigma_{(-j)} \Big) \\
 &= \Pr \Big(  \WWRowCon_\edge \,  a_{\edge}  \leq 3 \gamma  \Sigma_{(-j)} + \gamma \WWRowCon_\edge \,  a_{\edge}(\Point) \Big) \\
 &\leq \Pr \Big(  \WWRowCon_\edge \,  a_{\edge}(\Point)  \leq 3 \gamma  \left( \Sigma_{(-j)} + \WWRowCon_\edge \,  a_{\edge}(\Point) \right)\Big) \\
&= \Pr(\g{\Input} \leq 3 \gamma),
\end{align*}
and this concludes the proof for the upper bound. The argument for the lower bound is symmetric in that it uses the lower bound $\hat{\Sigma}_{(-j)} \ge (1 - \epsilon) \Sigma_{(-j)}$ and upper bound  $a_{\edge}(\Point)(1+\epsilon) \ge \hat a_{\edge}(\Point)$ instead in conjunction with the fact that $\nicefrac{1-\epsilon}{1 + \epsilon} \ge 1/3$ for $\epsilon \in (0,1/2)$.
\end{proof}

We now combine Lemmas~\ref{lem:order-statistic-sampling} and \ref{lem:cdf-relationship} to establish our main result of the section.
%which establishes that a poly-logarithmic (in $1/\delta$ and $\eta \cdot \eta^*$) sized $\SS \subseteq \PP$ suffices to obtain $\Pr_{\Point \sim \DD} \left(\exists{\edge \in \Wpm} : C \, \s < \g{\Input} \right) \leq \frac{\delta |\Wpm|} {4 \eta \, \eta^*}$.
%
%
%
\begin{theorem}[Empirical Sensitivity Approximation]
\label{thm:sensitivity-approximation}
Let $\epsilon \in (0,1/2), \delta \in (0,1)$, $\ell \in \compressiblelayers$, Consider a set $\SS = \{\Point_1, \ldots, \Point_n\} \subseteq \PP$ of size $|\SS| = \SizeOfS$ such that $\hat a^{\ell-1}(\Point') \in (1 \pm \epsilon) a^{\ell-1}(\Point')$ for all $\Point' \in \SS$. Then, 
$$
\Pr_{\Point \sim \DD} \left(\exists{\edge \in \Wpm} : C \, \s < \gHat{\Input} \right) \leq \frac{\delta |\Wpm|} {4 \eta \, \eta^*},
$$
where $C = \Cdef \ge 9 K$ and $\Wpm \subseteq [\eta^{\ell-1}]$.
\end{theorem}
\begin{proof}
Consider an arbitrary $\edge \in \Wpm$ and $\Input' \in \SS$ corresponding to $\g{\Input'}$ with CDF $\cdf{\cdot}$ and recall that $M = \min \{x \in [0,1] : \cdf{x} = 1\}$ as in Assumption~\ref{asm:cdf}. Let $\hat{M} = \min \{x \in [0,1] : \cdfHat{x} = 1\}$ be the analogous bound for the CDF associated with our relative importance approximation $\gHat{\Input}$. 

Invoking Lemma~\ref{lem:cdf-relationship}, we have $
\cdfHat{3 \, M} \geq \cdf{M} = 1$. Thus, $\hat{M} \leq 3 M$ by definition of $\hat{M}$. Now, we have
\begin{align*}
\cdfHat{\nicefrac{\hat{M}}{C}} &\leq \cdfHat{\nicefrac{3 \, M}{C}} &\text{Since $\hat{M} \leq 3 M$} \\
&\leq \cdf{\nicefrac{9 \, M}{C}} &\text{By the upper bound of Lemma~\ref{lem:cdf-relationship}} \\
&\leq \cdf{\nicefrac{M}{K}} &\text{Since $C \ge 9 K$} \\
&\leq \exp(-1/K) &\text{By Assumption~\ref{asm:cdf}}.
\end{align*}

Thus we have shown that the random variables $\gHat{\Input'}$ for $\Input' \in \SS$ satisfy the CDF condition required by Lemma~\ref{lem:order-statistic-sampling}. Thus, invoking Lemma~\ref{lem:order-statistic-sampling}, we obtain
\begin{align*}
\Pr(C \, \s < \gHat{\Input} ) &= \Pr \left(C \, \max_{\Point' \in \SS} \gHat{\Input'} < \gHat{\Input} \right) \\
&\leq \exp(-|\SS|/K).
\end{align*}
Since our choice of $\edge \in \Wpm$ was arbitrary, the bound applies for any $\edge \in \Wpm$. Thus, we have by the union bound
\begin{align*}
\Pr(\exists{\edge \in \Wpm} \,: C \, \s < \gHat{\Input}) &\leq \sum_{\edge \in \Wpm} \Pr(C \, \s < \gHat{\Input} ) \\
&\leq \abs{\Wpm} \exp(-|\SS|/K) \\
&= \left(\frac{|\Wpm|}{\eta^*} \right) \frac{\delta}{4 \eta},
\end{align*}
and this concludes the proof.
%The proof for bounding the probability of the complementary $\Aminus^\compl$ proceeds in the exact same manner and yields
% \begin{align*}
% \Pr(\Aminus^\compl) &\leq \abs{\Wminus} \exp(-|\SS|/K).
% \end{align*}
% Putting it all together, we have by the union bound, by $K \leq \kmax$, and the fact that $|\SS| = \SizeOfS$,
% \begin{align*}
% \Pr(\Aminus \cap \Aplus) &= 1 - \Pr(\Aminus^\compl \cup \Aplus^\compl) \\
% &\ge 1 - \left(\Pr(\Aminus^\compl) + \Pr(\Aplus^\compl \right) \\
% &\ge 1 - \exp(-|\SS|/K) \left(\abs{\Wmi} + \abs{\Wpm} \right) \\
% &\ge 1 - \exp(-|\SS|/K) \eta^{\ell-1} \\
% &\ge 1 - \left(\frac{\eta^{\ell-1}}{\eta^*} \right) \frac{\delta}{4 \eta} \\
% &\ge 1 - \frac{\delta}{4 \eta},
% \end{align*}
% and this concludes the theorem.
\end{proof}

In practice, the set $\SS$ referenced above is chosen to be a subset of the original data points, i.e., $\SS \subseteq \PP$ (see Alg.~\ref{alg:main}, Line~\ref{lin:s-construction}). Thus, we henceforth assume that the size of the input points $|\PP|$ is large enough (or the specified parameter $\delta \in (0,1)$ is sufficiently large) so that $|\PP| \ge |\SS|$.

\CB{TODO: Move this over to Importance Sampling Section}
\CB{Don't we need this to hold for the maximum $\DeltaNeuron$ over all $i \in [\eta^\ell]$????????}
\begin{lemma}[Empirical $\DeltaNeuronTrue$ Approximation]
\label{lem:delta-hat-approx}
Let $\delta \in (0,1)$, $\lambdaStar = \lambdamax$, and define 
$$
\DeltaNeuronHat = \DeltaNeuronHatDef,
$$
where $\kappa = \kappaDef$ and $\SS \subseteq \PP$ is as in Alg.~\ref{alg:main}. Then,
$$
\Pr_{\Point \sim \DD } \left(\max_{\neuron \in [\eta^\ell]} \DeltaNeuron[\Point] \leq \DeltaNeuronHat \right) \ge 1 - \frac{\delta}{4 \eta}.
$$
\end{lemma}
\begin{proof}
Define the random variables $\YY_{\Point'} = \E[\DeltaNeuron[\Point']] - \DeltaNeuron[\Point']$ for each $\Point' \in \SS$ and consider the sum $$
\YY = \sum_{\Point' \in \SS} \YY_{\Point'} = \sum_{\Point' \in \SS} \left(\E[\DeltaNeuron[\Point]] - \DeltaNeuron[\Point']\right).
$$
We know that each random variable $\YY_{\xx'}$ satisfies $\E[\YY_{\xx'}] = 0$ and by Assumption~\ref{asm:subexponential}, is subexponential with parameter $\lambda \leq \lambdaStar$. Thus, $\YY$ is a sum of $|\SS|$ independent, zero-mean $\lambdaStar$-subexponential random variables, which implies that $\E[\YY] = 0$ and that we can readily apply Bernstein's inequality for subexponential random variables~\cite{vershynin2016high} to obtain for $t \ge 0$
$$
\Pr \left(\frac{1}{|\SS|} \YY \ge t\right) \leq \exp \left(-|\SS| \, \min \left \{-\frac{t^2}{4 \, \lambdaStar^2}, \frac{t}{2 \, \lambdaStar} \right\} \right).
$$
Since $\SS = \SizeOfS \ge 2 \lambda^* \logTerm$, we have for $t = \sqrt{2 \lambdaStar}$,
\begin{align*}
\Pr \left(\E[\DeltaNeuron[\Point]] - \frac{1}{|\SS|} \sum_{\Point' \in \SS} \DeltaNeuron[\Point'] \ge t \right) &= \Pr \left(\frac{1}{|\SS|} \YY \ge t\right) \\
&\leq \exp \left( -|\SS| \frac{t^2}{4 \lambdaStar^2} \right) \\
&\leq \exp \left( - \logTerm  \right) \\
&= \frac{\delta}{\logTermInside}.
\end{align*}

Moreover, for single $\Point \sim \DD$, by the equivalent definition of a subexponential random variable~\cite{vershynin2016high}, we have for $u \ge 0$
$$
\Pr(\DeltaNeuron[\Point] - \E[\DeltaNeuron[\Point]] \ge u) \leq \exp \left(-\min \left \{-\frac{u^2}{4 \, \lambdaStar^2}, \frac{u}{2 \, \lambdaStar} \right\} \right).
$$
Thus, for $u = 2 \lambdaStar \, \logTerm$ we obtain
$$
\Pr(\DeltaNeuron[\Point] - \E[\DeltaNeuron[\Point]] \ge u) \leq \exp \left( - \logTerm  \right) = \frac{\delta}{ \logTermInside}.
$$
Therefore, by the union bound, we have with probability at least $1 - \frac{\delta}{4 \eta \, \eta^*}$:
\begin{align*}
	\DeltaNeuron[\Point] &\leq \E[\DeltaNeuron[\Point]]  + u \\
    &\leq \left(\frac{1}{|\SS|} \sum_{\xx' \in \SS} \DeltaNeuron[\Point'] + t \right) + u \\
    &= \frac{1}{|\SS|} \sum_{\Point' \in \SS} \DeltaNeuron[\Point'] + \left(\sqrt{2 \lambdaStar} + 2 \lambdaStar \, \logTerm \right) \\
    &= \frac{1}{|\SS|} \sum_{\Point' \in \SS} \DeltaNeuron[\Point'] + \kappa \\
    &\leq \DeltaNeuronHat,
\end{align*}
where the last inequality follows by definition of $\DeltaNeuronHat$.

Thus, by the union bound, we have
\begin{align*}
\Pr_{\Point \sim \DD } \left(\max_{\neuron \in [\eta^\ell]} \DeltaNeuron[\Point] > \DeltaNeuronHat \right) &= \Pr \left(\exists{\neuron \in [\eta^\ell]}: \DeltaNeuron[\Point] > \DeltaNeuronHat \right) \\
&\leq \sum_{\neuron \in \eta^{\ell-1}}  \Pr \left(\DeltaNeuron[\Point] > \DeltaNeuronHat \right) \\
&\leq \eta^{\ell-1} \left(\frac{\delta}{4 \eta \, \eta^*} \right) \\
&\leq \frac{\delta}{4 \, \eta},
\end{align*}
where the last line follows by definition of $\eta^* \ge \eta^{\ell -1}$.
\end{proof}
